# Supplementary material for: Quantifying mixed-state quantum entanglement by optimal entanglement witness
Source: arXiv:1203.1099 source file (2012-03-06)
Supplement: Supplementary file 1 [file MSE_supp.pdf]

# Supplementary information for 'Quantifying mixed-state quantum entanglement by optimal entanglement witness'

S.-S. B. Lee and H.-S. Sim
*Department of Physics, Korea Advanced Institute of Science and Technology, Daejeon 305-701, Korea*
(Dated: September 15, 2011)

### SLOCC invariance of extensive three-tangle

We show that three-tangle $\tau_3$ is not SLOCC invariant for mixed states, while the extensive three-tangle $\mathcal{T}_3$ is.

We discuss the condition that a measure $\mathcal{E}$, defined to be SLOCC invariant for pure states, is also invariant for mixed states under SLOCC operations $O$, $\mathcal{E}(\rho) = \mathcal{E}(O\rho O^\dagger)$. SLOCC operations do not conserve the normalization of states, $\langle\psi|O^\dagger O|\psi\rangle \neq \langle\psi|\psi\rangle$ in general. On the other hand, the convex roof construction, $\mathcal{E}(\rho) = \inf_{\{p_i,\psi_i\}} \sum_i p_i\ \mathcal{E}(|\psi_i\rangle)$, is defined for normalized states, $\mathrm{Tr}(\rho) = 1$ and $\langle\psi_i|\psi_i\rangle = 1$. To see the invariance, one needs to study the dependence of $\mathcal{E}$ on the normalization.

We apply the above discussion to three-tangle $\tau_3$; see Ref. [25] of the main text. For pure states $\psi$, $\tau_3$ is SLOCC invariant, $\tau_3(O|\psi\rangle) = \tau_3(|\psi\rangle)$, and it has the quadratic dependence on the normalization $\langle\psi|\psi\rangle$,

$$\tau_3(|\psi\rangle) = \langle\psi|\psi\rangle^2 \tau_3(|\psi\rangle/\sqrt{\langle\psi|\psi\rangle}).$$

For mixed states, $\tau_3$ is extended via Eq. (1), and has the same quadratic dependence, $\tau_3(\rho) = (\mathrm{Tr}\rho)^2\tau_3(\rho/\mathrm{Tr}\rho)$. Due to this, $\tau_3$ is not SLOCC invariant for mixed states.

To see this in details, we consider a pure-state decomposition of a mixed state, $\rho = \sum_i p_i \pi_{\psi_i}$, where $\pi_{\psi_i} = |\psi_i\rangle\langle\psi_i|$ and $\mathrm{Tr}\rho$, $\sum_i p_i$, $\mathrm{Tr}\pi_{\psi_i} = 1$. For this decomposition, the convex sum of $\tau_3$ is $\sum_i p_i \tau_3(|\psi_i\rangle)$. We also consider a SLOCC transformed state $\tilde\rho = O\rho O^\dagger$. The normalized state $\tilde\rho/\mathrm{Tr}\tilde\rho$ is

$$\frac{O\rho O^\dagger}{\mathrm{Tr}(O\rho O^\dagger)} = \frac{1}{\mathrm{Tr}(O\rho O^\dagger)}\sum_i p_i O\pi_{\psi_i}O^\dagger,$$
$$= \sum_i \tilde q_i \underbrace{\frac{O\pi_{\psi_i}O^\dagger}{\mathrm{Tr}(O\pi_{\psi_i}O^\dagger)}}_{\text{normalized}}, \qquad \tilde q_i \equiv \frac{p_i \mathrm{Tr}(O^\dagger O \pi_{\psi_i})}{\mathrm{Tr}(O\rho O^\dagger)}.$$

One notices $\sum_i \tilde q_i = 1$. The convex sum of $\tau_3$ for this decomposition is $\sum_i \tilde q_i \tau_3(\frac{O|\psi_i\rangle}{\sqrt{\langle\psi_i|O^\dagger O|\psi_i\rangle}})$. We rewrite it as

$$\sum_i \tilde q_i \tau_3(\frac{O|\psi_i\rangle}{\sqrt{\langle\psi_i|O^\dagger O|\psi_i\rangle}}) = \sum_i \frac{p_i \tau_3(|\psi_i\rangle)}{\langle\psi_i|O^\dagger O|\psi_i\rangle \mathrm{Tr}(O\rho O^\dagger)},$$

where we have used $\tau_3(|\psi\rangle) = \langle\psi|\psi\rangle^2\tau_3(|\psi\rangle/\sqrt{\langle\psi|\psi\rangle})$, the SLOCC invariance of $\tau_3$ for pure states, and the relation between $\tilde q_i$ and $p_i$. This convex sum for $\tilde\rho/\mathrm{Tr}\tilde\rho$ is *not* proportional to the convex sum $\sum_i p_i\tau_3(|\psi_i\rangle)$ for $\rho$ in general. Hence, it is unlikely to have a simple relation between $\tau_3(\rho)$ and $\tau_3(O\rho O^\dagger)$.

For example, we consider the convex mixture $\rho_{\mathrm{GW}}(p) = (1-p)\pi_{\mathrm{GHZ}} + p\pi_{\mathrm{W}}$ in Eq. (7) and a SLOCC transformation of the mixture, $\tilde\rho(p) = O_t \rho_{\mathrm{GW}}(p) O_t^\dagger$ with $O_t = \left(\begin{smallmatrix} t & 0 \\ 0 & t^{-1}\end{smallmatrix}\right)^{\otimes 3}$. We compute $\tau_3(\rho_{\mathrm{GW}})$ and $\tau_3(\tilde\rho)$ [$= (\mathrm{Tr}\tilde\rho)^2\tau_3(\tilde\rho/\mathrm{Tr}\tilde\rho)$] by using the optimal witness, and find $\tau_3(\tilde\rho) \neq \tau_3(\rho_{\mathrm{GW}})$ in general. For instance, for $p = 0.2$ and $t = 2$, $\tau_3(\rho_{\mathrm{GW}}) = 0.460$ and $\tau_3(\tilde\rho) = 0.386$. This shows that $\tau_3$ is not SLOCC invariant for mixed states.

Contrary to $\tau_3$, extensive three-tangle $\mathcal{T}_3$ is extensive as $\mathcal{T}_3(r\pi_\psi) = r\mathcal{T}_3(\pi_\psi)$ for positive real $r$, hence, $\mathcal{T}_3(|\psi\rangle) = \langle\psi|\psi\rangle\mathcal{T}_3(|\psi\rangle/\sqrt{\langle\psi|\psi\rangle})$. Because of this, $\mathcal{T}_3$ is SLOCC invariant for mixed states, $\mathcal{T}_3(\rho) = \mathcal{T}_3(O\rho O^\dagger)$.

### General form of the optimal witness for $\mathcal{T}_3$

We offer a rigorous proof of the general form in Eq. (4) in two steps. We first derive the form, and then show that the form does not overestimate $\mathcal{T}_3$ for all pure states. We also discuss the features of $\Pi$.

Theorem 1 ensures that any optimal witness $X_\rho$ should be optimal also for at least one pure state $\psi$ in GHZ\W class, $\mathrm{Tr}(X_\rho|\psi\rangle\langle\psi|) = \mathcal{T}_3(|\psi\rangle)$. In addition to this relation, we use the optimality of $X_\rho$. As in Fig. S1, $\mathrm{Tr}(X_\rho\rho) = \mathcal{T}_3(\rho)$ provides the tangent hyperplane to the SLOCC orbit $O\rho O^\dagger$. Since $\mathrm{Tr}(X_\rho O\rho O^\dagger)$ is maximal at $O = I$ in the orbit ($I$ is the identity), one has

$$\mathrm{Tr}(X_\rho\rho) = \mathrm{Tr}(X_\rho(I+\delta O)\rho(I+\delta O)^\dagger)$$

up to the first order of an infinitesimal SLOCC operation $\delta O$. We apply this to $\rho = \pi_\psi$, since $X_\rho$ is optimal for $\psi$, and obtain $\mathrm{Tr}(X_\rho\delta O\pi_\psi) + \mathrm{Tr}(X_\rho\pi_\psi\delta O^\dagger) = 0$. By representing $\delta O$ in terms of Pauli matrices and applying the relation of $|\psi\rangle = \sqrt{\mathcal{T}_3(|\psi\rangle)}O_\psi|\mathrm{GHZ}\rangle$ in Eq. (3), one rewrites the optimality condition as the nine equations of $\mathrm{Tr}(O_\psi^\dagger X_\rho O_\psi \Sigma_{ij}\pi_{\mathrm{GHZ}}) = 0$, where $j = 1,2,3$ is the local qubit index, $\Sigma_{i1} = \sigma_i\otimes I_2\otimes I_2$, $\Sigma_{i2} = I_2\otimes\sigma_i\otimes I_2$, $\Sigma_{i3} = I_2\otimes I_2\otimes\sigma_i$, $\sigma_i$ is the Pauli matrix with $i = 1,2,3$, and $I_2$ is the $2\times 2$ identity. The solution of the nine equations has the form of $\langle\mathrm{GHZ}|O_\psi^\dagger X_\rho O_\psi \propto \langle\mathrm{GHZ}|$. Since $\mathrm{Tr}(X_\rho\pi_\psi) = \mathcal{T}_3(|\psi\rangle)$, the solution becomes $O_\psi^\dagger X_\rho O_\psi|\mathrm{GHZ}\rangle = |\mathrm{GHZ}\rangle$. This gives the general form in Eq. (4), in which $X_\rho$ has the GHZ projector $\pi_{\mathrm{GHZ}}$ and the other projectors $\Pi$ orthogonal to $\pi_{\mathrm{GHZ}}$. This form is applicable to lower-rank states, although it is derived for full-rank states with choosing the full Hilbert space $\mathcal{H}_{\mathrm{f}}$ for $\mathcal{H}$.

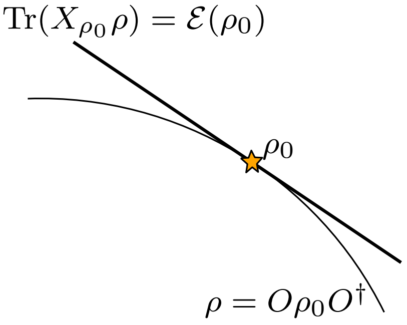


FIG. 1: Fig. S1. Optimal witness as the tangent hyperplane to a SLOCC orbit. $X_{\rho_0}$ is the optimal witness for a full-rank state $\rho_0$, $\mathrm{Tr}(X_{\rho_0}\rho_0) = \mathcal{T}_3(\rho_0)$, and the SLOCC orbit consists of the states $\rho = O^\dagger \rho_0 O$ obtained with varying a SLOCC operation $O$ continuously. The SLOCC invariance of $\mathcal{T}_3$ and the optimality of $X_{\rho_0}$ for $\rho_0$ ensure that $\mathrm{Tr}(X_{\rho_0}\rho) = \mathcal{E}(\rho_0)$ provides the tangent hyperplane to the SLOCC orbit at $\rho_0$.

Next, we prove that the form of $X_\rho$ in Eq. (4) does not overestimate $\mathcal{T}_3$ for all pure states. This is true for all W-class pure states, as one notices the relation of $\mu = \max_{\varphi \in \mathrm{W}} \langle \varphi | \pi_{\mathrm{GHZ}} + \Pi | \varphi \rangle$. It is also true for all GHZ\W-class pure states, as shown below. Without loss of generality, we put $O = I$ in the form in Eq. (4), because we consider all pure states and because $O|\psi\rangle$ can be treated as a pure state. Then a general form of the pure states, for which $X_\rho$ (with $O = I$) in Eq. (4) gives a positive expectation value, is written as $|\psi(p,\theta)\rangle = \sqrt{1-p}|\mathrm{GHZ}\rangle + \sqrt{p}e^{i\theta}|\phi\rangle$ where $\langle \phi|\mathrm{GHZ}\rangle = 0$, $p \in [0,1]$ and $\theta \in [0, 2\pi)$; $X_\rho$ does not overestimate $\mathcal{T}_3$ for those with a negative expectation value of $X_\rho$. We define the function $f(p) = \min_\theta \mathcal{T}_3(|\psi(p,\theta)\rangle)$, and notice that $f(p) \geq 1 - p/p_0$ in the range of $0 \leq p < p_0$ where $f(p)$ is nonzero. And, one can show that $\mathrm{Tr}(X_{\mathrm{GHZ}}\pi_{\psi(p,\theta)}) \leq 1 - p/p_0$ for all $\theta$ and $0 \leq p < p_0$. Therefore,

$$\mathrm{Tr}(X_{\mathrm{GHZ}}\pi_{\psi(p,\theta)}) \leq \mathcal{T}_3(|\psi(p,\theta)\rangle),$$

and $X_\rho$ in Eq. (4) does not exceed $\mathcal{T}_3$ for all pure states.

In addition, we discuss the form of $\Pi$ and $\mathbb{P}_{X_\rho}$. As mentioned in the main text, $\mathbb{P}_{X_\rho}$ possesses one GHZ\W-class pure state and the other W-class pure states $|\mathrm{Z}_i\rangle$'s. The states $|\mathrm{Z}_i\rangle$'s give the maximal overlap $\mu = \langle \mathrm{Z_i}|\pi_{\mathrm{GHZ}} + \Pi|\mathrm{Z_i}\rangle$, and $\langle \mathrm{Z_i}|\mathrm{Z_i}\rangle = 1$. It is likely that $|\mathrm{Z}_i\rangle$ is belonging to W \ BS class, i.e., neither biseparable (BS) nor separable, as W \ BS class has larger parameter space dimension than BS class. In this case, $|\mathrm{Z}_i\rangle$ should satisfy $O^\dagger_{\mathrm{Z_i}}(\pi_{\mathrm{GHZ}} + \Pi - \mu I)O_{\mathrm{Z_i}}|\mathrm{W}\rangle \propto |111\rangle$; $O_{\mathrm{Z_i}}$ is a SLOCC operator. This relation of $|\mathrm{Z}_i\rangle$ is obtained by using the W\BS-class state form of $|\mathrm{Z_i}\rangle \equiv O_{\mathrm{Z_i}}|\mathrm{W}\rangle$, SLOCC orbits, and the optimality of $X_\rho$. This relation of $|\mathrm{Z}_i\rangle$ is nontrivial, and only special forms of $\Pi$ satisfy that the number of $|\mathrm{Z}_i\rangle$'s in $\mathbb{P}_{X_\rho}$ is larger than one. We numerically study the point, by randomly selecting thousands of different forms of $\Pi$. Our numerical study might imply the following conjecture: The number of W-class states $|\mathrm{Z}_i\rangle$'s in $\mathbb{P}_{X_\rho}$ is larger than one, only if $\Pi$ is invariant under some of the symmetries of $\pi_{\mathrm{GHZ}}$ and $I$ such as permutation, exchange of qubit index, 0-1 flip, local phase rotations, or etc. It will be valuable to prove whether the conjecture is true. This conjecture is useful, when we consider states with $r_\rho > 2$, for which $\mathbb{P}_{X_\rho}$ should contain more than two pure states.

### Optimal pure-state decompositions of $\rho_{\mathrm{GI}}$ and $\rho_{\mathrm{GW}}$

We provide the optimal pure-state decomposition of $\rho_{\mathrm{GI}}$ and $\rho_{\mathrm{GW}}$ in Eqs. (5) and (7).

For $\rho_{\mathrm{GI}}$, the W-class mixed state $\rho_{\mathrm{Z}}$ is obtained as

$$\rho_{\mathrm{Z}} = \frac{1}{18}\sum_{\substack{s=\pm \\ m,n=0,1,2}} \pi_{\mathrm{Z}_{smn}},$$

where

$$|Z_{smn}\rangle = \left[\bigotimes_{\nu=m,n,-m-n} \begin{pmatrix} 1 & 0 \\ 0 & e^{i\frac{2\nu\pi}{3}} \end{pmatrix}\right] |Z_{s00}\rangle,$$
$$|\mathrm{Z}_{+00}\rangle = \sum_{i,j,k=0,1} a_{i+j+k}|ijk\rangle,$$
$$|\mathrm{Z}_{-00}\rangle = \sum_{i,j,k=0,1} a_{3-(i+j+k)}|ijk\rangle,$$

and $(a_0, a_1, a_2, a_3) \simeq (0.7436, -0.1750, -0.2133, 0.4677)$.

The optimal pure-state decomposition of $\rho_{\mathrm{GW}}$ is

$$\rho_{\mathrm{GW}}(p) = \begin{cases} \mathcal{T}_3(p)\pi_{\mathrm{GHZ}} + \dfrac{1-\mathcal{T}_3(p)}{3}\displaystyle\sum_{n=0,1,2}\pi_{\mathrm{Z}'_n(p_0)}, & p \leq p_0, \\ \dfrac{1}{3}\displaystyle\sum_{n=0,1,2}\pi_{\mathrm{Z}'_n(p)}, & p > p_0. \end{cases}$$

Here $|\mathrm{Z}'_n(p)\rangle = \sqrt{1-p}|\mathrm{GHZ}\rangle - \sqrt{p}\, e^{2n\pi i/3}|\mathrm{W}\rangle$ with $n = 0,1,2$ are W-class states with $\mathrm{Tr}(X_{\rho_{\mathrm{GW}}}\pi_{\mathrm{Z}'_n}) = 0$.

### Optimal witness for the geometric measure of entanglement

The geometric measure of entanglement $\mathcal{E}_{\mathrm{G}}$ [2] for pure state is given by

$$\mathcal{E}_{\mathrm{G}}(|\psi\rangle) = 1 - \max_{|s\rangle \in \mathbb{S}} |\langle \psi|s\rangle|^2, \tag{1}$$

where $\mathbb{S}$ is the set of separable states. Then we have the inequality that

$$\langle \psi|X|\psi\rangle \leq \langle \psi|X_\psi|\psi\rangle = \mathcal{E}_{\mathrm{G}}(|\psi\rangle) \leq 1 - |\langle \psi|s\rangle|^2, \tag{2}$$
$$1 \geq \langle \psi|(X + \pi_s)|\psi\rangle. \tag{3}$$

Here the equality holds when $X$ is optimal, $X = X_\psi$, and the separable state $|s\rangle$ gives the maximal overlap with $|\psi\rangle$. Therefore we get the optimality condition of witness as

$$\max_{|s\rangle\in\mathbb{S}} \lambda_{\max}[X + \pi_s] = 1, \quad (4)$$

where $\lambda_{\max}[\cdot]$ denotes the maximum eigenvalue.

The numerical recipe to find optimal witnesses for $\mathcal{E}_{\mathrm{G}}$ is quite straightforward; start from the initial candidate of witness $X^{(0)}$, then iteratively update the candidate $X^{(i)}$ at $i$-th step until $\lambda^{(i)} = \max_{|s\rangle\in\mathbb{S}} \lambda_{\max}[X^{(i)} + \pi_s]$ converges to unity. The next candidate at each step is chosen by the value of $\lambda^{(i)}$. If $\lambda^{(i)} > 1$, update $X^{(i+1)}$ such that

$$0 < X^{(i)} - X^{(i+1)} < \lambda^{(i)} - (1 - \mu^{(i)}), \quad (5)$$

and else if $\lambda^{(i)} < 1$,

$$0 < X^{(i+1)} - X^{(i)} < (1 + \mu^{(i)}) - \lambda^{(i)}, \quad (6)$$

where $\mu^{(i)} \in (0, 1)$ is the paramter controlling the convergence. As $\lambda^{(i)}$ approaches to unity, $\mu^{(i)}$ decreases. Note that the calculation of $\lambda^{(i)}$ requires the optimization over only pure separable states which occupy much less parameter space.

### Entanglement in noisy Smolin state

Smolin state [1] is four-qubit unlockable bound entangled state defined as

$$\rho_{\mathrm{S}} = \frac{1}{4}\sum_{i=1}^{4} \pi_{\varphi_i}, \quad (7)$$

where $|\varphi_i\rangle$'s are GHZ-like states : $|\varphi_1\rangle = (|0000\rangle + |1111\rangle)/\sqrt{2}$ and $|\varphi_i\rangle = s_1 s_i |\varphi_1\rangle$ for $i > 1$. Here $s_i$ denotes to take Pauli matrix $\sigma_x$ on $i$-th qubit. The bound entanglement in the Smolin state is quantified by the geometric measure of entanglement as 1/2 [3]. Though the Smolin state is experimentally realized in quantum optical setup [4], its reliability of boundness of its entanglement is poor since there are five negative eigenvalues over all three partial transpositions [6]. To ensure the boundness, noisy Smolin state [5], which is the mixture of Smolin state and white noise

$$\rho_{\mathrm{NS}}(p) = p\rho_{\mathrm{S}} + (1 - p)\frac{I}{16}, \quad (8)$$

is produced in a four-photon state [6]. While it is known that the noisy Smolin state is separable for $p \in [0, 1/3]$ and bound entangled for $p \in (1/3, 1]$ [5], its amount of entanglement is not considered yet. We quantify the bound entanglement of Smolin state using the geometric measure of entanglement.

First, we simplify the form of witness $X$ according to the common symmetries of $\rho_{\mathrm{NS}}$ and $\mathcal{E}_{\mathrm{G}}$. Exploiting the symmetries under the permutation of qubit indices and local unitary operations such as taking $\sigma_x$ on two qubits, taking $\sigma_z$ on two qubits, taking $\sigma_x^{\otimes 4}$, taking $\left(\begin{smallmatrix}1&0\\0&i\end{smallmatrix}\right)^{\otimes 4}$, and taking $[(\sigma_y + \sigma_z)/\sqrt{2}]^{\otimes 4}$, we see that there are only two independent real parameters of $X$ :

$$X = \alpha\left(\sum_{i=1}^{4} \pi_{\varphi_i}\right) + \beta\left(1 - \sum_{i=1}^{4} \pi_{\varphi_i}\right), \quad (9)$$

where $\alpha \geq 0$ and $\beta \leq 0$.

Defining $\mathrm{P}_\varphi \equiv \sum_{i=1}^{4} \pi_{\varphi_i} = 4\rho_{\mathrm{S}}$, any separable state is decomposed as $|s\rangle = \mathrm{P}_\varphi|s\rangle + (I - \mathrm{P}_\varphi)|s\rangle$. Then it is sufficient to condider the subspace spanned by $\mathrm{P}_\varphi|s\rangle$ and $(I - \mathrm{P}_\varphi)|s\rangle$ to get the maximum eigenvalue of $X + \pi_s$, that is,

$$\lambda_{\max}[X + \pi_s] = \lambda_{\max}\left[\begin{pmatrix} \alpha + q & \sqrt{q(1-q)}e^{i\theta} \\ \sqrt{q(1-q)}e^{-i\theta} & \beta + (1-q) \end{pmatrix}\right], \quad (10)$$

where the basis for RHS is $\{\mathrm{P}_\varphi|s\rangle, (I - \mathrm{P}_\varphi)|s\rangle\}$. Here $|s\rangle$ is parametrized as $\langle s|\mathrm{P}_\varphi|s\rangle = q$ and $\langle s|\mathrm{P}_\varphi|s\rangle\langle s|(I - \mathrm{P}_\varphi)|s\rangle = \sqrt{q(1-q)}e^{i\theta}$. Since $\alpha \geq 0$ and $\beta \leq 0$, the maximum eigenvalue is nondecreasing function of $q$. Straightforward algebraic calculation gives $q = \langle s|\mathrm{P}_\varphi|s\rangle \leq 1/2$ (see Appendix A in Ref. [3]). Therefore the relation between $\alpha$ and $\beta$ is obtained by equating RHS of Eq. (10) for $q = 1/2$ with unity,

$$\lambda_{\max}\left[\begin{pmatrix} \alpha + \frac{1}{2} & e^{i\theta}/2 \\ e^{-i\theta}/2 & \beta + \frac{1}{2} \end{pmatrix}\right] = 1, \quad (11)$$

resulting in two solutions $\alpha^{-1} + \beta^{-1} = 2$ and $\alpha = \beta = 0$.

Maximizing the expectation value $\mathrm{Tr}(X\rho_{\mathrm{NS}}(p)) = [(1 + 3p)\alpha + 3(1-p)\beta]/4$ for given $p$, we get the final result

$$\begin{aligned} \mathcal{E}_{\mathrm{G}}(\rho_{\mathrm{NS}}) &= [2 - \sqrt{3(1-p)(1+3p)}]/4 \\ \alpha &= [1 - \sqrt{3(1-p)/(1+3p)}]/2 \\ \beta &= [1 - \sqrt{(1+3p)/3(1-p)}]/2 \end{aligned} \quad (12)$$

for $p \in (1/3, 1]$ and $\mathcal{E}_{\mathrm{G}}(\rho_{\mathrm{NS}}) = \alpha = \beta = 0$ for $p \in [0, 1/3]$. Numerical approach introduced above reproduces this analytic solution well. Note that this result coincides with previous ones such as the full separability for $p \in [0, 1/3]$ [5] and $\mathcal{E}_{\mathrm{G}}(\rho_{\mathrm{S}}) = 1/2$ [3].

It is remarkable that, to quantify the bound entanglement of noisy Smolin state in experiment, only a single measurement result $\mathrm{Tr}(\mathrm{P}_\varphi\rho_{\mathrm{NS}}) = (1 + 3p)/4$ is enough. Even if the state is slightly deviated from the exact form of $\rho_{\mathrm{NS}}$, this analysis gives a successful lower bound of entanglement. As a realistic example, the experimental noisy Smolin entanglement produced in Ref. [6] can be quantified merely by using the experimentally measured

witness value $\langle\mathcal{W}\rangle = \mathrm{Tr}[(I - \sum_{i=1}^{3}\sigma_i^{\otimes 4})\rho_{\mathrm{NS}}]$. The "witnessed" amount of entanglement is given by

$$\mathcal{E}_{\mathrm{G}}^{(\mathrm{wit})}(\rho_{\mathrm{NS}}) = \max_{p\in[0,1]} \frac{\alpha(p)+\beta(p)}{2} - \frac{\alpha(p)-\beta(p)}{4}\langle\mathcal{W}\rangle, \tag{13}$$

and, for the data points in Ref. [6], it is clearly the lower bound of $\mathcal{E}_{\mathrm{G}}(\rho_{\mathrm{NS}}(p^{(\mathrm{est})}))$ where $p^{(\mathrm{est})}$ is the estimated value of $p$ from full state reconstruction via quantum state tomography.

[1] J. A. Smolin, Phys. Rev. A **63**, 032306 (2001).
[2] T.-C. Wei and P. M. Goldbart, Phys. Rev. A **68**, 042307 (2003).
[3] T.-C. Wei, J. B. Altepeter, P. M. Goldbart, and William J. Munro, Phys. Rev. A **70**, 022322 (2004).
[4] E. Amselem and M. Bourennane, Nature Phys. **5**, 748 (2009).
[5] R. Augusiak and P. Horodecki, Phys. Rev. A **74**, 010305(R) (2006).
[6] J. Lavoie, R. Kaltenbaek, M. Piani, and K. J. Resch, Phys. Rev. Lett. **105**, 130501 (2010).
